# Supplementary material for: A well-scaling natural orbital theory
Source: arXiv:1611.08692 ancillary file (2016-11-26)
Supplement: Supplementary file 1 [file Supporting_Information_new.pdf]

# Supporting Information:

A well-scaling natural orbital theory

by R. Gebauer, M. H. Cohen, and R. Car

## S1. SIGNS FOR POSITIVE MATRIX ELEMENTS

The proof of the sign conjecture for positive matrix elements utilizes NSO-based Brillouin-Wigner perturbation theory (BWPT). An SD basis is constructed from the NSOs of the true ground-state wave function $\Psi_G$ of $\hat{H}$, which has parts diagonal, $\hat{H}^d$, and off-diagonal, $\hat{U}^{od}$, in the basis. $\hat{U}^{od}$ is the off-diagonal part of the $N$-electron Coulomb interaction. The eigenfunctions of $\hat{H}^d$ are the SD $\Phi_{\mathbf{n}}$, and $E_{\mathbf{n}}$ are the corresponding eigenvalues. $E_{\mathbf{0}} = \inf\{E_{\mathbf{n}}\}$ is the lowest of those and $\Phi_{\mathbf{0}}$ the associated eigenfunction. $\hat{U}^{od}$ is treated as a perturbation on $\hat{H}^d$; it generates $\Psi_G$ from $\Phi_{\mathbf{0}}$. The expansion coefficients $C_{\mathbf{n}}$ of $\Psi_G$ in the $\Phi_{\mathbf{n}}$ are

$$C_{\mathbf{n}} = C_{\mathbf{0}}\,\delta_{\mathbf{n},\mathbf{0}} + (1-\delta_{\mathbf{n},\mathbf{0}})\sum_{\mathbf{l}\neq\mathbf{n}}\left[E_G - E_{\mathbf{l}}\right]^{-1}\left(\hat{U}^{od}\right)_{\mathbf{nl}} C_{\mathbf{l}}. \quad \textbf{[S1]}$$

The $a^{th}$-order term in the expansion of $C_{\mathbf{n}}$, $\mathbf{n}\neq\mathbf{0}$, is obtained by iterating Eq. **S1**:

$$C_{\mathbf{n}}^{(a)} = \sum_{\mathbf{l}_1\cdots\mathbf{l}_{a-1}}\left[E_G - E_{\mathbf{l}_{a-1}}\right]^{-1}\left(\hat{U}^{od}\right)_{\mathbf{n}\mathbf{l}_{a-1}}\cdots \cdots\left[E_G - E_{\mathbf{l}_1}\right]^{-1}\left(\hat{U}^{od}\right)_{\mathbf{l}_1\mathbf{0}} C_{\mathbf{0}}. \quad \textbf{[S2]}$$

Setting the sign of each $C_{\mathbf{n}}$ equal to that of the lowest order term in its BWPT expansion, the $a(\mathbf{n})^{th}$ term, is a variational approximation for the ground state. Whether the expansion converges is irrelevant, as only the formal structure of the lowest-order term is used. An excited NSO is one present in $\Phi_{\mathbf{n}}$ and not in $\Phi_{\mathbf{0}}$. Classify $C_{\mathbf{n}}$ by the number of its occupied excited NSOs and assign values $l \leq N$ to the index $l$ if $\psi_l$ is present in $\Phi_{\mathbf{0}}$ and $l > N$ if excited from $\Phi_{\mathbf{0}}$. Give $r_l$ the value 0 when $l \leq N$ and 1 when $l > N$. $R(\mathbf{n}) = \sum_{l\in\mathbf{n}} r_l$ is the number of excited NSOs in $\Phi_{\mathbf{n}}$ obtained by counting the number of indices $> N$ in $\mathbf{n}$. The PDC restricts $R(\mathbf{n})$ to be either odd or even for all $\mathbf{n}$. If $C_{\mathbf{0}}$ is finite, $R(\mathbf{n})$ must be even, $\forall\mathbf{n}$, as $R(\mathbf{0}) = 0$. In the lowest order $a(\mathbf{n})$ of $C_{\mathbf{n}}$, each matrix element on the right hand side of Eq. **S2** increases the values of 2 distinct $r_l$ from 0 to 1. Consequently

$$a(\mathbf{n}) = \frac{1}{2}R(\mathbf{n}),$$

each of the $a(\mathbf{n})$ matrix elements having changed 2 indices from $\leq N$ to $> N$. As each matrix element in Eq. **S2** is positive and denominator negative because $E_G < E_{\mathbf{n}}, \quad \forall \mathbf{n} \neq \mathbf{0}$, we obtain

$$\operatorname{sgn}\{C_{\mathbf{n}}\} = (-1)^{a(\mathbf{n})} = (-1)^{\frac{1}{2}R(\mathbf{n})} \qquad \text{[S3]}$$

as our variational approximation. Eq. **S3** implies that the sign $s(ii'\mathbf{m})$ of the coefficient $C_{ii'\mathbf{m}}$ is

$$s(ii'\mathbf{m}) = (-1)^{\frac{1}{2}R(ii'\mathbf{m})}. \qquad \text{[S4]}$$

$R(ii'\mathbf{m})$ can be decomposed into contributions from $ii'$ and from $\mathbf{m}$:

$$R(ii'\mathbf{m}) = R(ii') + R(\mathbf{m}). \qquad \text{[S5]}$$

$R(ii'\mathbf{m})$ is even. Eqs. **S4** and **S5** imply that

$$s(ii'\mathbf{m}) = (-1)^{\frac{1}{2}[R(ii')+R(\mathbf{m})]}.$$

The product of two signs in [**12**] becomes

$$s(ii'\mathbf{m})s(jj'\mathbf{m}) = (-1)^{\frac{1}{2}[R(ii')+R(jj')]}(-1)^{R(\mathbf{m})}. \qquad \text{[S6]}$$

$R(ii')$ and $R(\mathbf{m})$ must both be even or both odd. If $R(ii')$ is even, so must be $R(\mathbf{m})$ and therefore $R(jj')$. If $R(ii')$ is odd, so must be $R(\mathbf{m})$ and therefore $R(jj')$. With this added information, Eq. **S6** implies that

$$s(ii'\mathbf{m})s(jj'\mathbf{m}) = (-1)^{\frac{1}{2}[R(ii')+R(jj')]}(-1)^{\mathbb{P}(ii'\text{or } jj')}, \qquad \text{[S7]}$$

with

$$\mathbb{P}(ii'\text{or } jj') = \begin{cases} 0 & R(ii') \text{ and } R(jj') \text{ even} \\ 1 & R(ii') \text{ and } R(jj') \text{ odd} \end{cases}$$

$\mathbb{P}(ii'\text{or } jj')$ can be partitioned into $\frac{1}{2}\mathbb{P}(ii') + \frac{1}{2}\mathbb{P}(jj')$. Inserting this into Eq. **S7** proves the conjecture **13** with

$$s(ii') = (-1)^{\frac{1}{2}[R(ii')+\mathbb{P}(ii')]} \qquad \text{[S8]}$$

$$s(jj') = (-1)^{\frac{1}{2}[R(jj')+\mathbb{P}(jj')]}, \qquad \text{[S9]}$$

$R(ii')$ or $R(jj')$ can take only 3 values: 0, 1, and 2. The resulting signs are

| $R(ii')$ | $\mathbb{P}(ii')$ | $s(ii')$ |
|---|---|---|
| 0 | 0 | $+$ |
| 1 | 1 | $-$ |
| 2 | 0 | $-$ |

*Table S1. Sign rule for positive matrix elements*

As derived, Eqs. **S8**–**S9** and Table S1 apply to the signs of the coefficients in the expansion of the ground state $\Psi_G$ in SD comprised of the NSO of $\Psi_G$. Our goal is to find a sign rule for the coefficients in the expansion **1** of the trial function $\Psi$. We do so by making an arbitrary association of each NSO with index $i$ of $\Psi$ with an NSO of the same index $i$ of $\Psi_G$. If the NSO $i$ is considered occupied in $\Psi_G$, its associated NSO is considered "occupied" in $\Psi$ as well, and similarly for unoccupied NSOs. We now make the variational approximation that the signs $s(ii'\mathbf{m})$ of each $C(ii'\mathbf{m})$ in the expansion **1** of the trial function $\Psi$, are identical to the signs of the lowest-order terms of the corresponding coefficients $C(ii'\mathbf{m})$ in the expansion of the true ground state $\Psi_G$. It follows that Eqs. **S8** and **S9** and Table S1 then apply as well to the signs of the coefficients in the expansion of the trial function. Eqs. **S8**–**S9** and Table S1 thus constitute our sign rule. It is simple, variational, and of algebraic complexity, scaling as $M^2$. The rule was derived from three assumptions: (1) The PDC was imposed on the SD basis for expanding the ground state. (2) Each trial-function coefficient $C(ii'\mathbf{m})$ was given the sign of the lowest order term in the BWPT series of the corresponding ground-state coefficient. (3) All matrix elements $K_{ii',jj'} - K_{ii',j'j}$ are positive in the bases generated both by the ground-state and the trial-function NSOs. The rule is exact in the limit of weak correlation under the PDC, and its validity extends beyond that limit. There are 4 pairs of values for $R(ii')$ and $R(jj')$: $(0,0)$; $(0,2)$; $(1,1)$; $(2,2)$. The product $s(ii')s(jj')$ is negative only in the $(0,2)$ case, implying that the excitation of pairs is the primary driver by which correlation lowers the energy below the Hartree-Fock value, an intuitively obvious result.

*Signs in OP-NOFT-0:* All matrix elements are positive in OP-NOFT-0, and the PDC holds. All pairs are of the form i+,i- and can be labeled by the NO index $i$ alone, simplifying the sign notation to $\mathsf{s}(i) \equiv s(i+,i-)$. The lowest-order approximation yields the following

values of $\mathsf{s}(i)$

| $i \gtrless N/2$ | $\mathsf{s}(i)$ |
|---|---|
| $\leq$ | $+$ |
| $>$ | $-$ |

*Table S2. Sign rule for OP-NOFT-0*

Our search for the ground-state energy starts by constructing a random set of $M$ putative NOs labeled by $i = 1 \cdots M$. The OP-NOFT-0 sign rule assigns particular signs $\mathsf{s}(i)$ to the spin paired NSOs constructed from these randomly selected NOs according to the value of $i$ via Table S2. For the results of the search to be consistent with the internal logic of the derivation of the rule, in particular its relation to BWPT, the final results for the 1-OPs should obey the relation $p_1(i) \geq p_1(j)$ for $i \leq N/2$ and $j > N/2$, which we always find to be the case. In other words, fixing the initial sign of a NO, forces it to converge properly either to a “pseudo-occupied” or to a “pseudo-unoccupied” type of NO. In those computations in which the $\mathsf{s}(i)$ were assigned randomly, independent of the value of $i$, at convergence there were $N/2$ NO with positive $\mathsf{s}(i)$ with all others negative, in precise agreement with the sign rule of Table S2.

## S2. MINIMIZATION OF THE ENERGY

The minimization of the energy functional $E$ in [**29**] of the main text is performed using a damped Car-Parrinello dynamics approach. The NOs $\{\phi_i\}$ are propagated in ’time’ $t$ (the relaxation time) according to

$$\frac{d^2}{dt^2}|\phi_i\rangle = |F_i\rangle - \gamma \frac{d}{dt}|\phi_i\rangle + \sum_j \Lambda_{ij} S|\phi_j\rangle, \qquad \textbf{[S10]}$$

where $\gamma$ is a damping coefficient, the $\Lambda_{ij}$ are Lagrange multipliers that enforce orthonormality of the NOs, and $S$ is the overlap matrix. The generalized force $|F_i\rangle$ is defined as

$$|F_i\rangle = |g_i\rangle - \frac{1}{2}\sum_j \left(\langle\phi_j|g_i\rangle + \langle\phi_i|g_j\rangle\right) S|\phi_j\rangle.$$

The vectors $|g_i\rangle$ are given by $|g_i\rangle = -\frac{\partial E}{\partial\langle\phi_i|}$. This definition of $|F_i\rangle$ ensures that the forces lead to a quasi-unitary rotation within the space of the NO’s. The small loss of orthogonality accumulated in one time step is corrected by the Lagrange multipliers.

The occupation probabilities $p_1$ and $p_{11}$ are written as

$$\begin{aligned} p_1(i) &= \frac{1}{2}\left(\mathrm{erf}(x(i)) + 1\right) \\ p_{11}(ij) &= \mathrm{SUP} + (p_1(<) - \mathrm{SUP})\left(\mathrm{erf}(X(ij)) + 1\right), \end{aligned}$$

where SUP is defined as $\sup\left(p_1(i) + p_1(j) - 1, 0\right)$. The parameters $x(i)$ and $X(ij)$ vary from $-\infty$ to $+\infty$. This functional form automatically satisfies the bounds for $p_{11}$ and for $p_1$ given, respectively, in [**9**] and below [**5**] of the main text.

The $x(i)$ and $X(ij)$ are optimized simultaneously with the NO's by damped dynamics equations similar to Eq. **S10**, in which Lagrange multipliers enforce the sum rules for the $p_1$ and the $p_{11}$. The condition **10** of the main text is imposed by adding a penalty function to the energy functional.

Typically the infimum of the functional is reached after a few thousand steps. No effort was made to optimize this protocol.

## S3. DISSOCIATION CURVES FOR DIMERS $H_2$, LIH, AND HF

In the following, we show the dissociation curves for three dimers, obtained at various levels of theory. Notice that for $H_2$ we used the larger cc-pVTZ basis set.

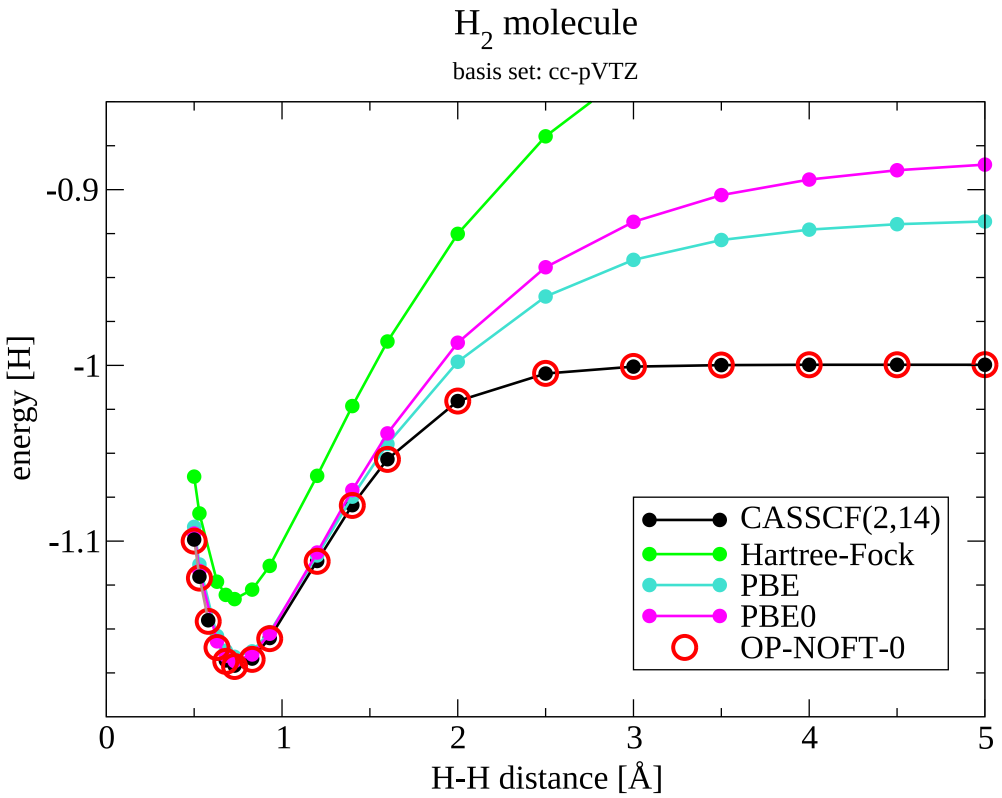


*FIG. S1. Dissociation curve of $H_2$.*

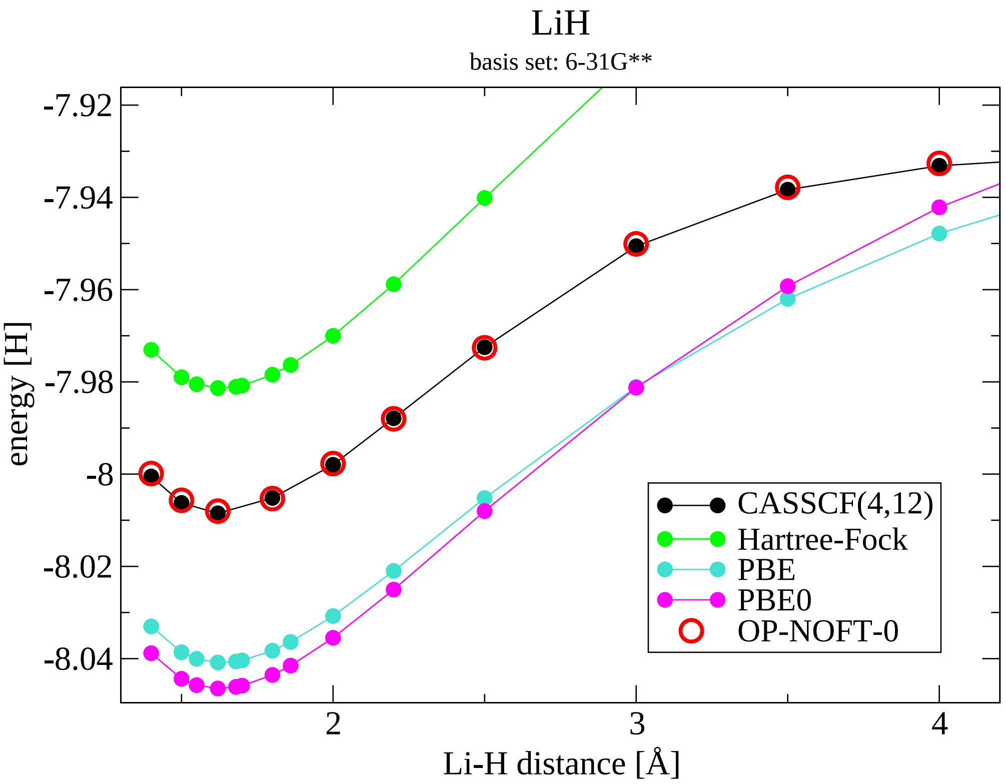


*FIG. S2. Dissociation curve of LiH.*

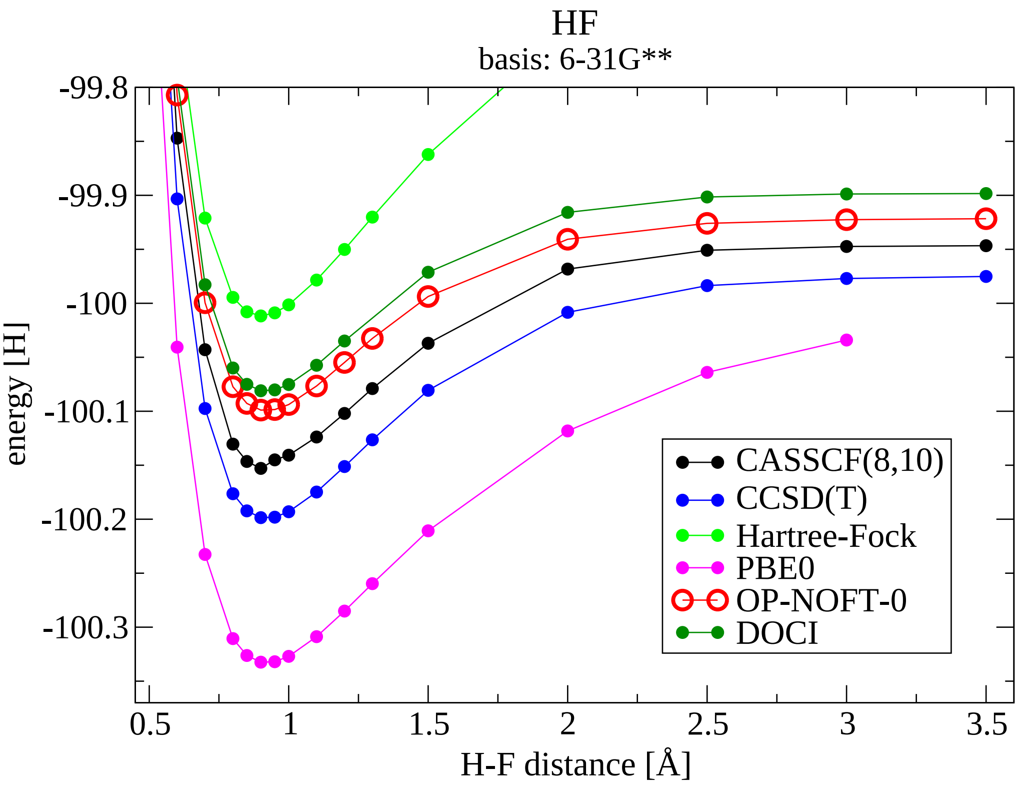


*FIG. S3. Dissociation curve of HF.*

Our results for the binding energies of HF are given in Table S3:

| **Method** | **Binding energy (eV)** |
|---|---|
| CCSD(T) | 6.08 |
| CASSCF(8,10) | 5.61 |
| DOCI | 4.97 |
| OP-NOFT-0 | 4.82 |

*Table S3. Computed binding energies of HF*

The optimized OP-NOFT-0 NOs were used as the basis in the DOCI computations. The CCSD(T) result is close to the experimental value of 6.06 $\pm$ 0.2 eV [S1]. Our OP-NOFT-0 result differs from our DOCI result by only 0.15 eV, and both differ from CCSD(T) and experiment by $\sim$ 1eV.

The discrepancies from DOCI for HF and $N_2$ are larger than for our other test molecules. They are the only test molecules in which there is more than one active occupied orbital in the separated parts at the Hartree-Fock level. As we have seen that adding a higher positivity

condition does not affect the results, we conclude that the error relative to DOCI comes from the $\xi$ approximation for $N > 4$ and gets worse as that number of orbitals increases. Ayers, Scuseria, and their collaborators have found that in molecules like HF and $N_2$ the AP1roG/Pair-CCD method [S2-S4] is almost visually indistinguishable from DOCI and has the same scaling as OP-NOFT-0 [S5]. However, an important feature of our formulation is that it offers ways to explore systematic improvement of the $\xi$-approximation and to go beyond DOCI by introducing more generalized pairing with expectation of improved accuracy while retaining $N^3$ scaling.

## S4. CONDITIONS FOR TWO-STATE PROBABILITIES IN 4-ELECTRON SYSTEMS

The conditions given in [**9**]–[**11**] of the main text apply to systems with more than four electrons. In the case of four electrons (like, e.g. LiH), each determinant in the $A = 0$ sector is made of two doubly occupied states. In this case, the conditions on the two-state OPs are:

$$\sup(p_1(i) + p_1(j) - 1, 0) \leq p_{11}(ij) \leq p_1(<)$$
$$\sum_{j(\neq i)} p_{11}(ij) = p_1(i),$$

where $p_1(<)$ is the lesser of $p_1(i)$ and $p_1(j)$.

## S5. PALDUS $H_4$ TEST

In 1980 Jankowski and Paldus introduced [S6] a model to test various approaches for strongly correlated electron systems. This model consists of three series of 4-electron systems where the geometry of an arrangement of four hydrogen atoms is varied using a single parameter $\alpha$. In the three series, the four atoms are arranged in a trapezoidal (H4), rectangular (P4), and linear (D4) configuration, respectively. In Fig. S4 we depict the three configurations.

In order to test the OP-NOFT-0 functional in these configurations, we used a minimal basis set of one s-like function on each hydrogen atom (STO-6G). We performed full CI (FCI) calculations, as well as double-occupancy CI (DOCI), where the single particle orbitals

were chosen as the Hartree-Fock orbitals (DOCI@HF) or the natural orbitals obtained from minimizing the OP-NOFT-0 functional (DOCI@NO). The correlation energies are reported in Table S4. The third column of Table S4 lists the DOCI correlation energies obtained when the converged OP-NOFT-0 NOs are used as basis functions. The results are identical within numerical accuracy to those of OP-NOFT-0, showing that the signs are exact and that OP-NOFT-0 obtains DOCI results with algebraic complexity. The second column shows DOCI results obtained using converged Hartree-Fock orbitals that are somewhat worse than those of the 3rd column, implying that the converged OP-NOFT-0 NOs provide a more efficient basis of given finite size. DOCI and OP-NOFT-0 recover only a variable fraction of the FCI correlation energy.

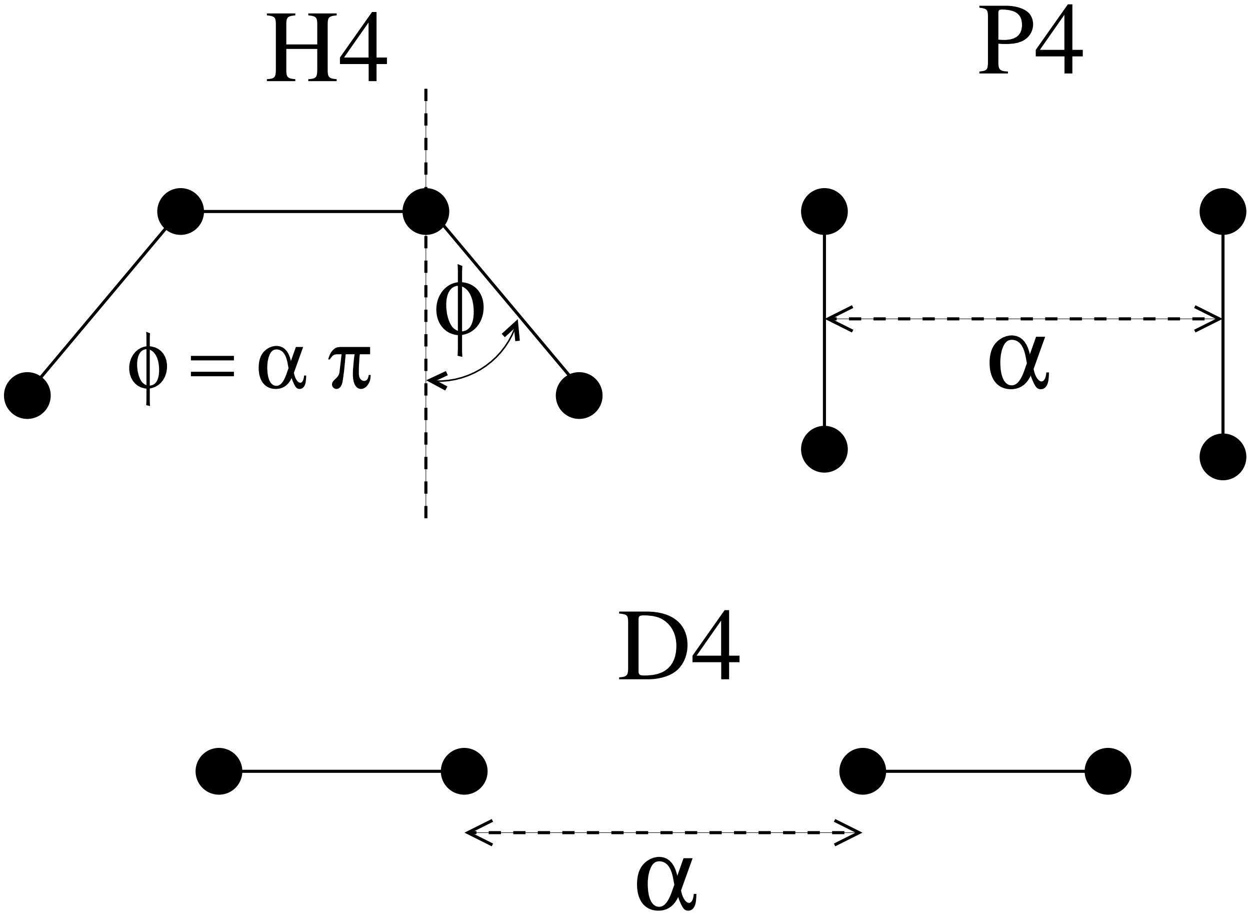


*FIG. S4. Geometry of the H4, P4, and D4 configurations in the Paldus test. Hydrogen atoms are depicted with black circles. The solid lines indicate a fixed H-H distance of $2a_0$ (corresponding to a stretched $H_2$ molecule). Each geometry is varied using a parameter $\alpha$ as shown.*

| $\alpha$ | $E_{corr}$(FCI) | $E_{corr}$(DOCI@HF) | $E_{corr}$(DOCI@NO) | $E_{corr}$(OP-NOFT-0) |
|---|---|---|---|---|
| **H4** | | | | |
| 0.005 | -0.1523398 | -0.0725544 | -0.0726629 | -0.0726629 |
| 0.015 | -0.1353406 | -0.0593798 | -0.0596758 | -0.0596757 |
| 0.020 | -0.1290278 | -0.0556022 | -0.0559236 | -0.0559236 |
| 0.050 | -0.1067682 | -0.0455382 | -0.0458908 | -0.0458908 |
| 0.100 | -0.0909272 | -0.0405894 | -0.0411607 | -0.0411607 |
| 0.200 | -0.0801374 | -0.0386401 | -0.0397021 | -0.0397021 |
| 0.500 | -0.0766017 | -0.0383718 | -0.0398523 | -0.0398523 |
| **P4** | | | | |
| 2.002 | -0.1628781 | -0.0829956 | -0.0829980 | -0.0829980 |
| 2.020 | -0.1562118 | -0.0761640 | -0.0761669 | -0.0761669 |
| 2.100 | -0.1341372 | -0.0578854 | -0.0578939 | -0.0578939 |
| 2.200 | -0.1183235 | -0.0484987 | -0.0485393 | -0.0485394 |
| 4.000 | -0.0813502 | -0.0271051 | -0.0271051 | -0.0271051 |
| 10.000 | -0.0792859 | -0.0223087 | -0.0223087 | -0.0223087 |
| **D4** | | | | |
| 1.000 | -0.0996238 | -0.0802154 | -0.0873200 | -0.0873200 |
| 1.500 | -0.0827506 | -0.0537729 | -0.0582650 | -0.0582650 |
| 2.000 | -0.0766017 | -0.0383684 | -0.0398523 | -0.0398523 |
| 4.000 | -0.0791365 | -0.0250104 | -0.0250245 | -0.0250245 |
| 6.000 | -0.0793186 | -0.0231395 | -0.0231399 | -0.0231399 |

*Table S4. Correlation energies from Paldus $H_4$ test. All energies in Hartrees.*

## S6. OCCUPATION NUMBERS AND ENTANGLEMENT ENTROPY

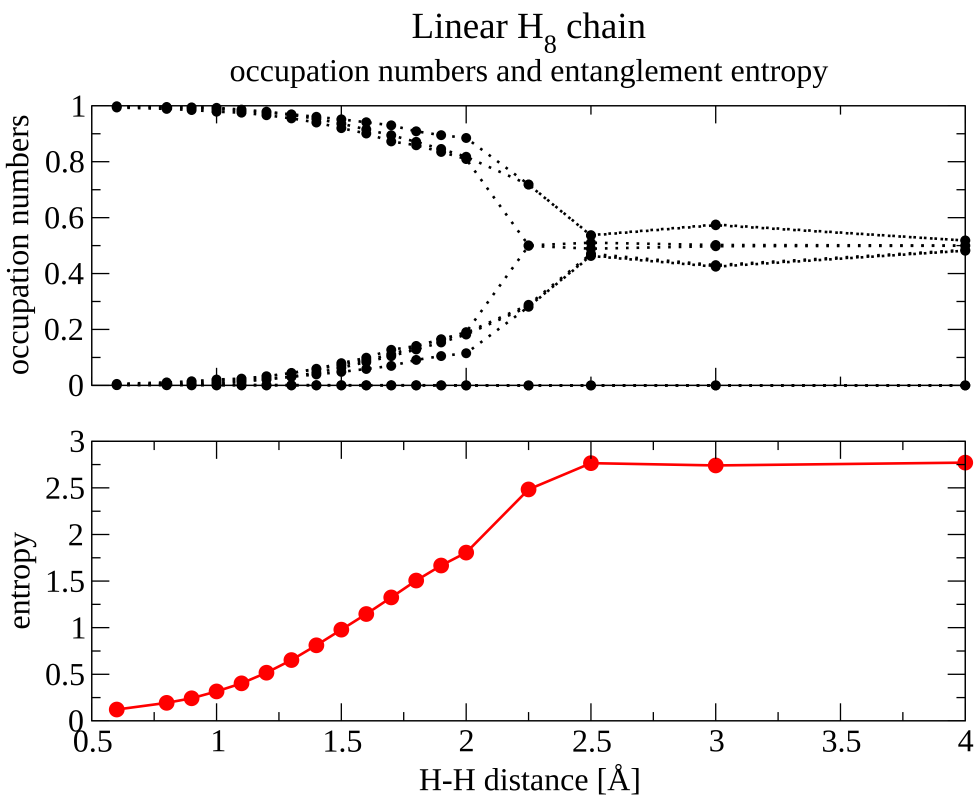


*FIG. S5. Occupation numbers and Von Neumann entanglement entropy in $H_8$ as a function of interatomic distance.*

## S7. PAIR-CORRELATION FUNCTION

The parallel spin and anti-parallel spin pair-correlation functions $g_p(\mathbf{r},\mathbf{r}') = g_{\sigma\sigma}(\mathbf{r},\mathbf{r}')$ and $g_a(\mathbf{r},\mathbf{r}') = g_{\sigma\bar{\sigma}}(\mathbf{r},\mathbf{r}')$ are defined as

$$n_\sigma(\mathbf{r})n_{\sigma'}(\mathbf{r}')g_{\sigma\sigma'}(\mathbf{r},\mathbf{r}') = \pi(\mathbf{r}\sigma,\mathbf{r}'\sigma';\mathbf{r}\sigma,\mathbf{r}'\sigma'), \qquad \textbf{[S11]}$$

where $n_\sigma(\mathbf{r}) = \frac{1}{2}\rho(\mathbf{r},\mathbf{r})$. Plots of the pair correlation functions for the symmetric open-bounded $H_8$ chain are given in Fig. S6. These depict $g$ for electrons of opposite and parallel spins when one electron is placed in the mid-bond (left panel), and in the mid-antibond (right panel). We notice that the anti-parallel spin correlation shows a positive hump at the location of the tagged electron (dashed vertical line), contrary to what one should expect for a repulsive cusp condition. This is an artifact of the use a of a finite Gaussian basis, as an

infinite set of NO's would be required to exactly reproduce the electron-electron cusp [S7]. For the stretched chain in Fig. S6 (H-H distance = 1.8 Å) the electron-electron cusp has negligible effect on the energy. We find a different behavior near equilibrium (H-H distance = 0.9 Å, plot not shown), where the hump gets replaced by a shallow local minimum of the pair correlation function at coalescence, i.e. a behavior qualitatively in agreement with the strong repulsive interaction between two electrons at short distance. These results are independent of the other approximations made and hold also for $H_4$ where our formula for $\xi$ is exact.

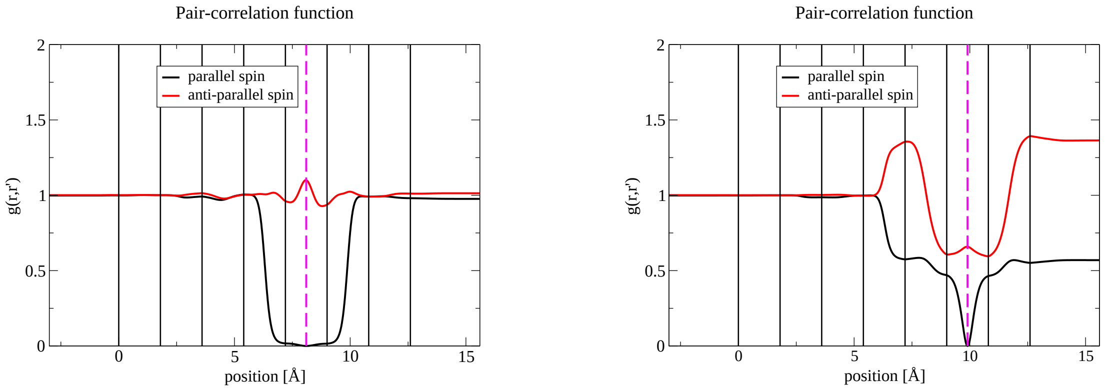


*FIG. S6. Electronic pair-correlation function along the $H_8$ axis when one electron is placed at the position of the vertical dashed line on the molecular axis. The vertical black lines show the atom positions. Left panel: one electron at mid-bond. Right panel: one electron at mid-antibond. The H-H distance is 1.8 Å .*

Fig. S7 depicts the pair-correlation function when one electron is placed outside the molecule's right end. An asymmetric exchange-correlation hole associated with the charging of the end atom can clearly be seen. The alternating bonding/antibonding character of the links between adjacent atoms is also manifest. This reflects the instability of the open chain toward a dimerizing distortion and is evident in the pair correlations when an electron resides respectively in the mid-bond or in the mid-antibond, as shown in Fig. S6, left and right panels respectively.

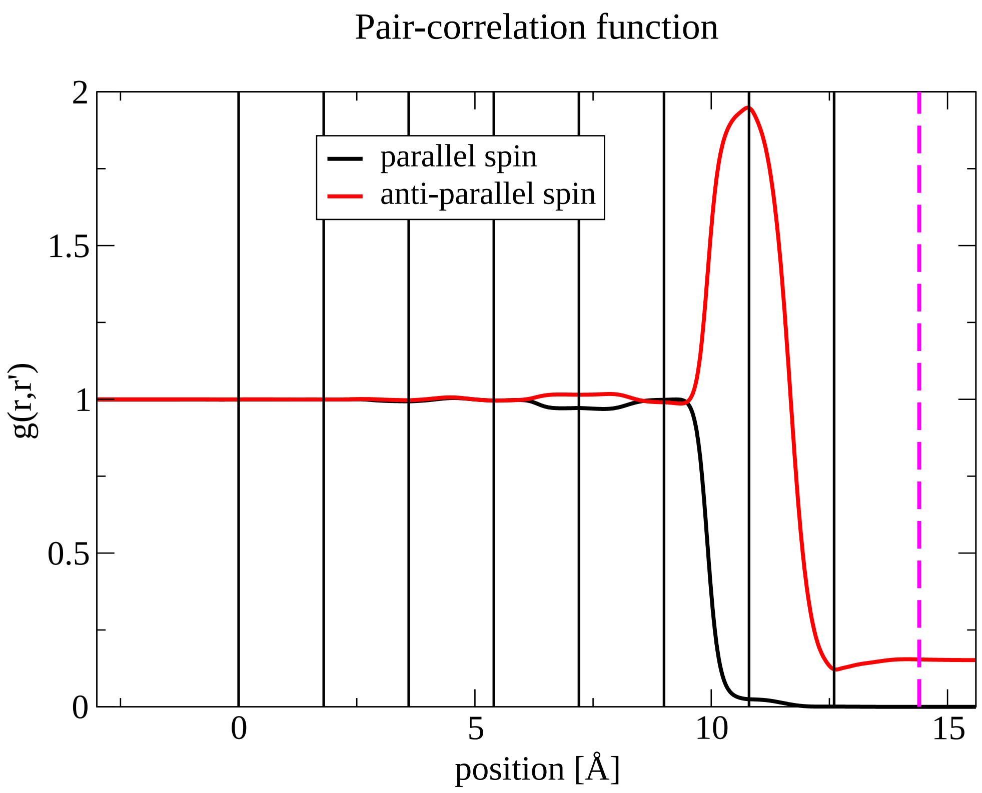


*FIG. S7. Electronic pair-correlation function along the $H_8$ axis when one electron is placed at the position of the vertical dashed line on the molecular axis. The vertical black lines show the atom positions. The H-H distance is 1.8 Å.*

## S8. ACRONYMS

| | |
|---|---|
| 1-DM | One-particle reduced density matrix |
| 2-DM | Two-particle reduced density matrix |
| 6-31G** | Pople's notation for a double-zeta split-valence Gaussian basis set |
| AP1roG/Pair-CCD | Antisymmetric product of geminals with one distinct "reference orbital" occupied in each geminal. See [S2-S4]. |
| BWPT | Brillouin-Wigner perturbation theory |
| CASSCF(n,m) | Complete active space self-consistent field with $n$ electrons in $m$ active orbitals |
| CCSD(T) | Coupled cluster with single, double, and perturbative triple electron-hole excitations |
| cc-pVTZ | Correlation consistent valence triple-zeta Gaussian basis set with polarization functions |
| CI | Configuration interaction |
| DFT | Density functional theory |
| DOCI | Doubly occupied configuration interaction |
| FCI | Full configuration interaction |
| NO | Natural orbital |
| NSO | Natural spin orbital |
| OC | Orthogonality constraint |
| OP | Single or joint natural-spin-orbital occupation probability |
| OP-NOFT | Occupation probability-based natural-orbital functional theory |
| OP-NOFT-0 | OP-NOFT restricted to seniority zero |
| n-OP or q-OP | single or joint NSO occupation probability; $n, q = 1, 2, \cdots, N$ |
| PBE | Semi-local exchange-correlation functional from Ref. 24 |
| PBE0 | Hybrid functional from Ref. 25 |
| PDC | Pair difference constraint |

| | |
|---|---|
| QMA | Quantum-Merlin-Arthur problems in complexity theory |
| SD | Slater determinant |
| SI | Online supporting information |
| STO-6G | Slater-type basis functions expressed with six contracted Gaussian functions |

**References:**

[S1] Gaydon AG (1953) *Dissociation Energies* (Chapman and Hall, London).

[S2] Limacher PA, Ayers PW, Johnson PA, De Baerdemacker S, Van Neck D, Bultinck P (2013) *A New Mean-Field Method Suitable for Strongly Correlated Electrons: Computationally Facile Antisymmetric Products of Nonorthogonal Geminals.* J. Chem. Theory Comp. 9:1394.

[S3] Johnson PA, Limacher PA, De Baerdemacker S, Van Neck D, Bultinck P (2013) *A size-consistent approach to strongly correlated systems using a generalized antisymmetrized product of nonorthogonal geminals.* Comput. Theor. Chem 1003:101-113.

[S4] Henderson TM, Bulik IW, Stein T, Scuseria GE (2014) *Seniority-based coupled cluster theory.* J. Chem. Phys. 141(24):244104.

[S5] Limacher PA, et al. (2014) *Simple and inexpensive perturbative correction schemes for antisymmetric products of nonorthogonal geminals.* Phys. Chem. Chem. Phys. 16(11):5061.

[S6] Jankowski K, Paldus J (1980) *Applicability of coupled-pair theories to quasidegenerate electronic states: A model study.* Int. J. Quantum Chem. 18(5):1243-1269.

[S7] Giesbertz KJH, van Leeuwen R (2013) *Natural occupation numbers: When do they vanish?* J. Chem. Phys. 139(10):104109.
